# Supplementary material for: Socratic Planner: Self-QA-Based Zero-Shot Planning for Embodied Instruction Following
Source: arXiv:2404.15190 source file (2025-03-26)
Supplement: Supplementary file 1 [file Appendix.tex]

\clearpage
\section*{Appendix}
\setcounter{section}{0}

\noindent Within this supplementary material, we provide additional details and experimental results that are not included in the main text due to space constraints.
\begin{itemize}
    \item~\cref{Appendix1}: Additional details for Socratic Planner, including each component’s prompt.
    \item~\cref{Appendix2}: Details of \textit{Relaxed}HLP mechanism 
    \item~\cref{Appendix3}: Additional Model implementation details
    \item~\cref{Appendix4}: Backbone agnostic experimental results
    \item~\cref{Appendix5}: Limitation of Socratic Planner and low-level controller with some failure cases
    \item~\cref{Appendix6}: Potential avenues for future work
\end{itemize} 
%%%
\section{Prompt Generators}
\label{Appendix1}
\begin{figure}[!t]
\centerline{\includegraphics[width=\columnwidth]{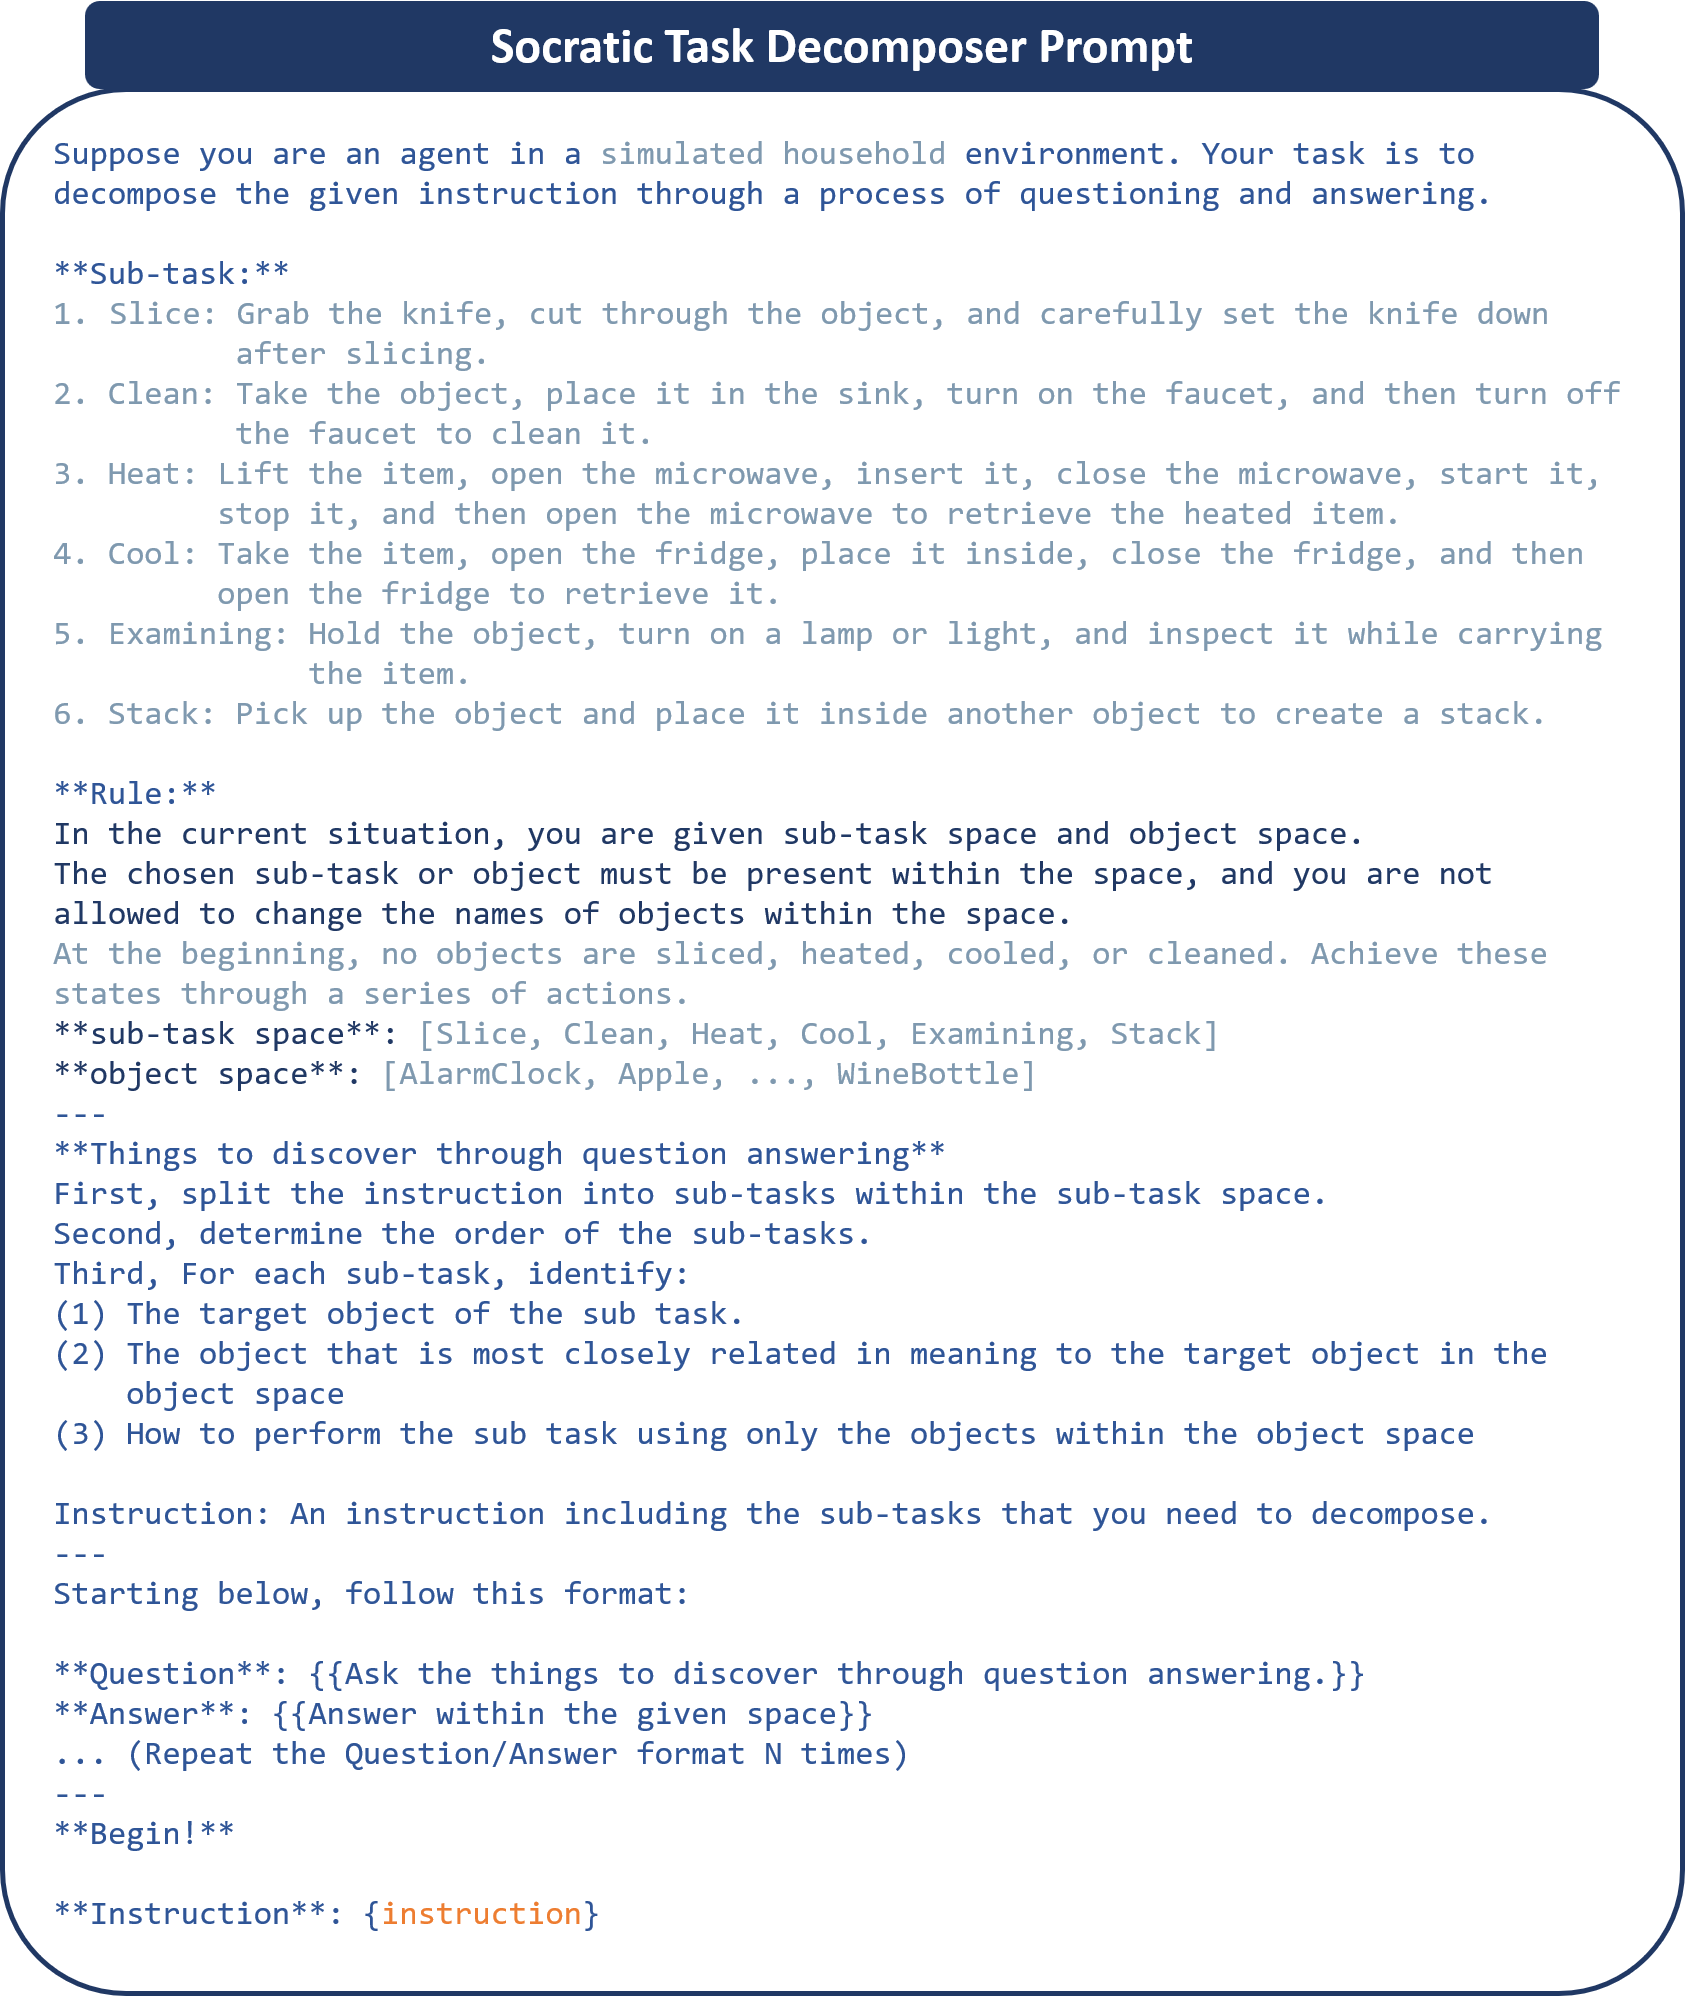}}
    \caption{Socratic Task Decomposer Prompt}
    \label{fig:socratic_task_decomposer_prompt} 
\end{figure}
\subsection{LLM prompt}
\subsubsection{Socratic Task Decomposer}
The prompt of the Socratic Task Decomposer for Socratic Planner is shown in~\cref{fig:socratic_task_decomposer_prompt}. 
The \textit{``\{instruction\}''} in~\cref{fig:socratic_task_decomposer_prompt} is replaced with the specific instruction.
\subsubsection{Task Planner}
The Task Planner's prompt is shown in~\cref{fig:task_planner_prompt}. 
The \textit{``\{instruction\}''} in the prompt is replaced with the specific instruction in the same way as STD.
Replace \textit{``\{QA\}''} with a QA conversation generated from STD.
For the experiments without STD, the task planner remains the same, except for the QA-related part as shown in~\cref{fig:task_planner_w_o_std_prompt}.
%%%
\begin{figure}[!t]
\centerline{\includegraphics[width=\columnwidth]{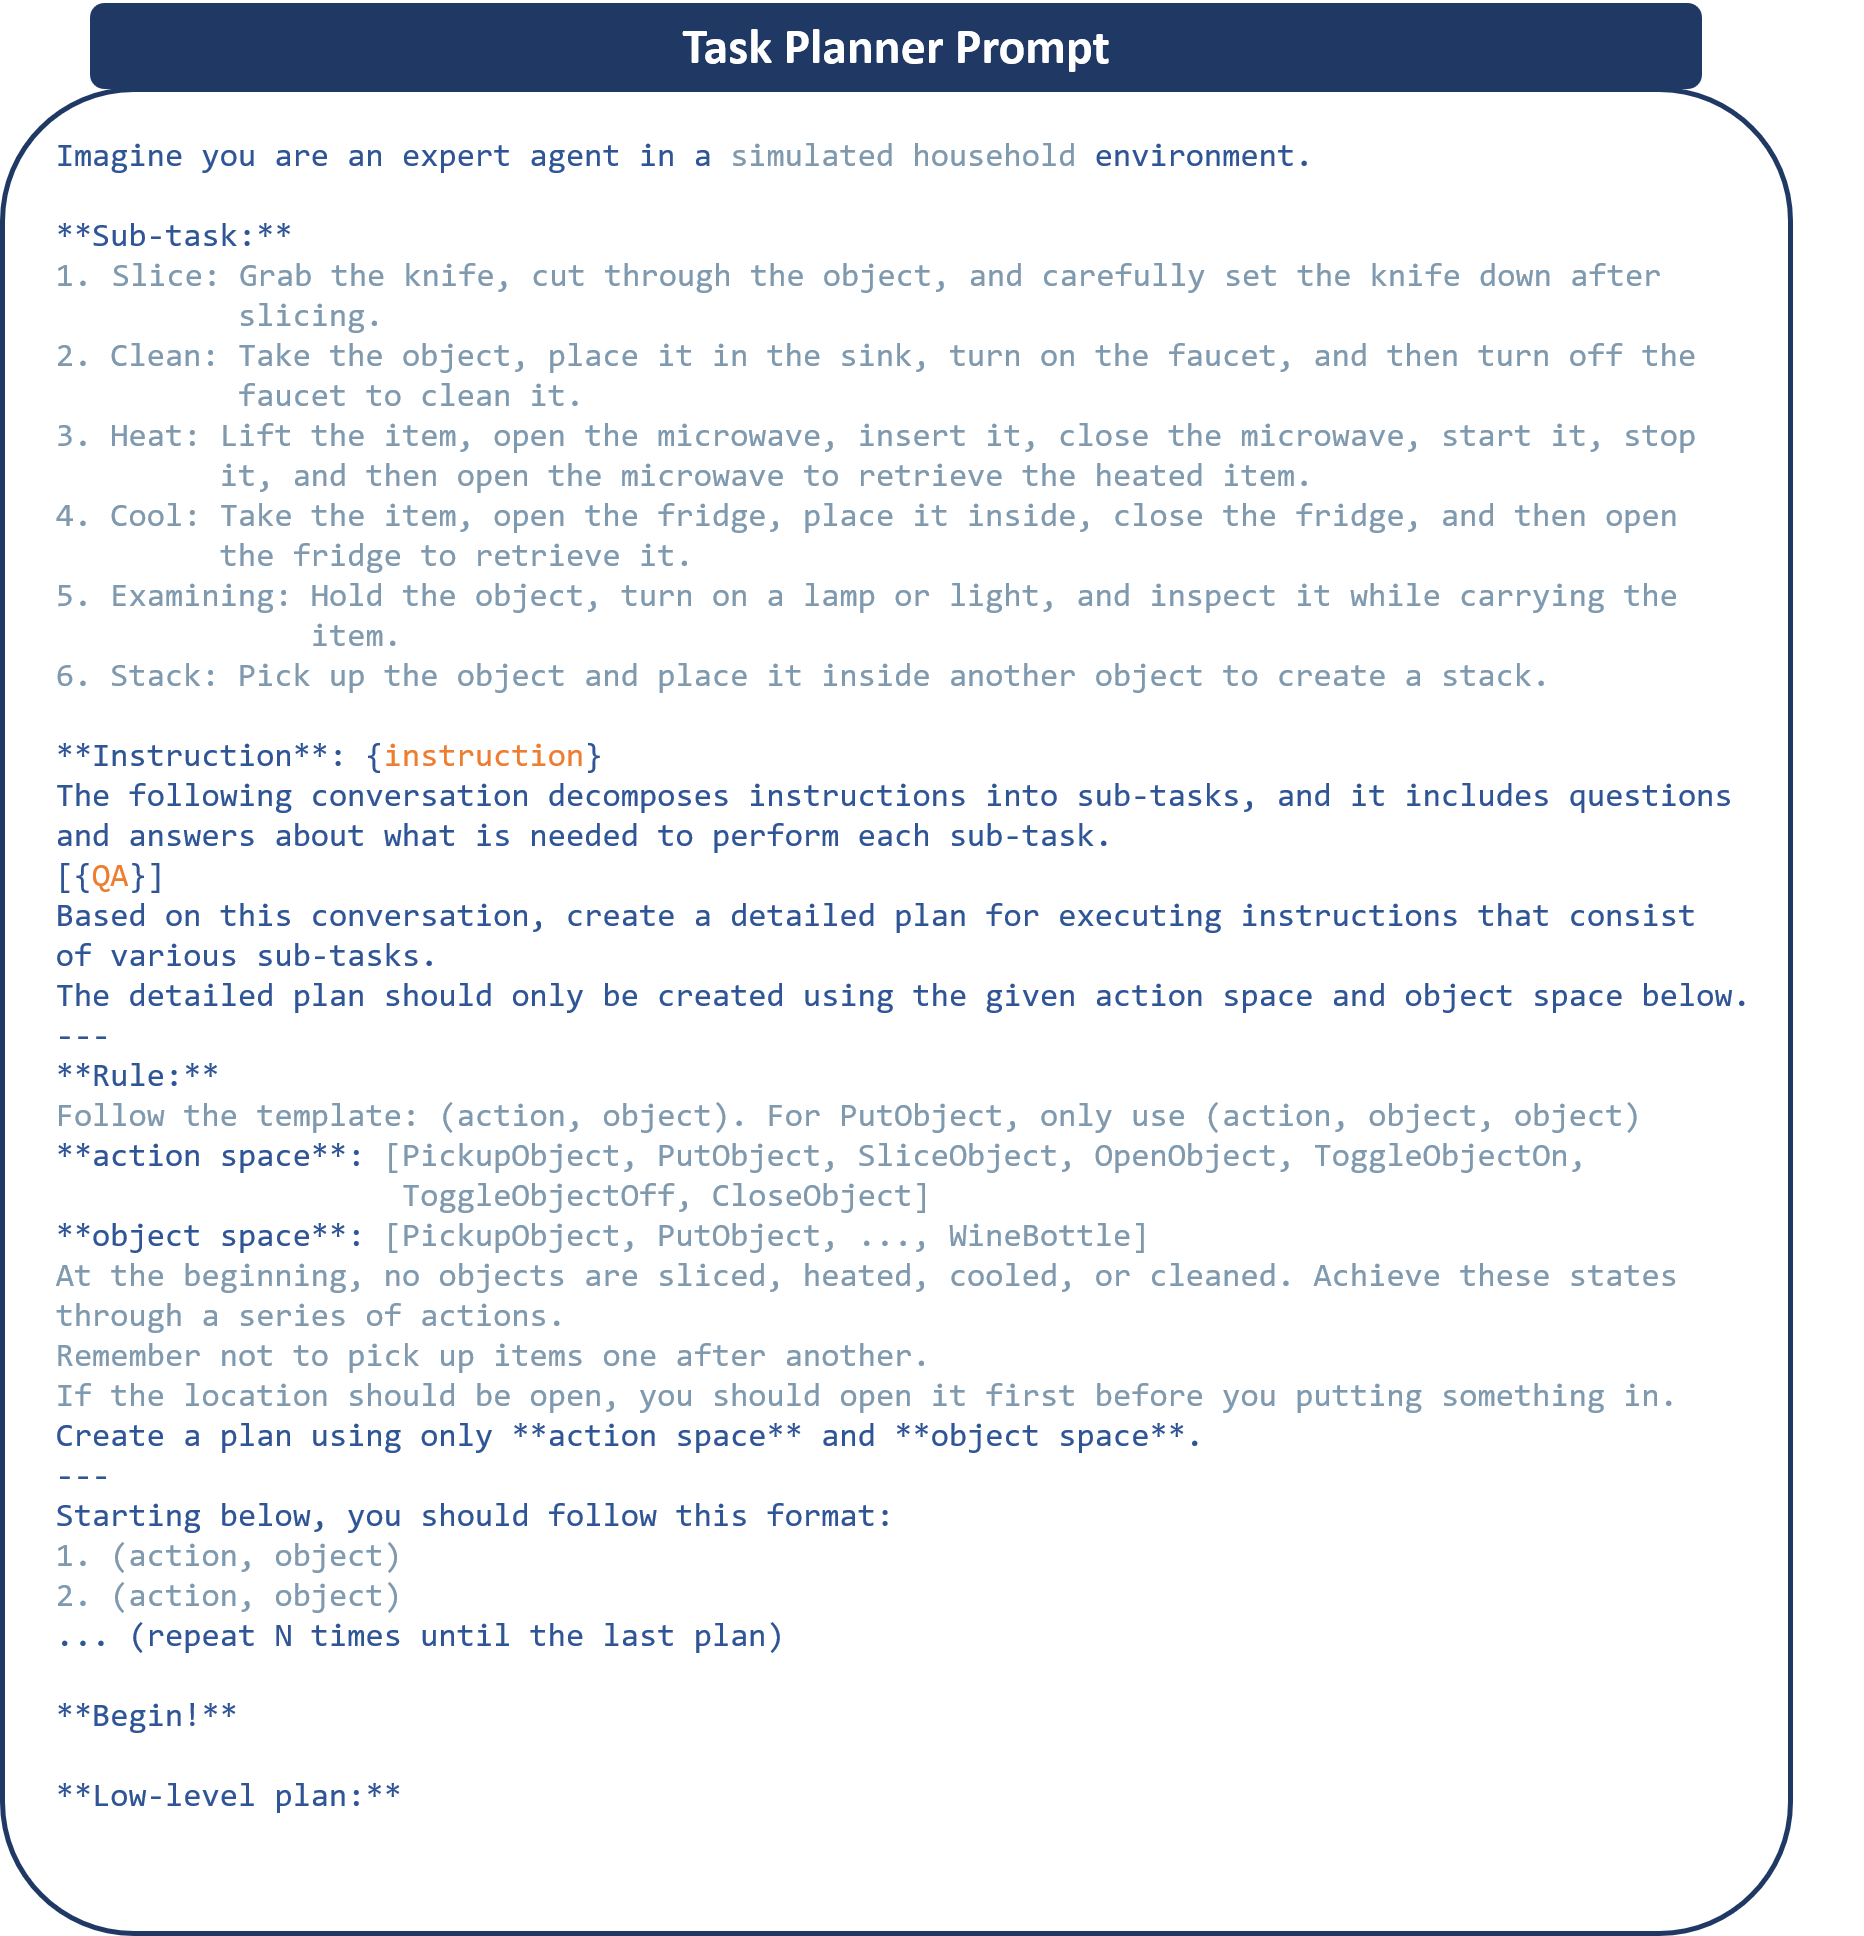}}
    \caption{Task Planner Prompt}
    \label{fig:task_planner_prompt} 
\end{figure}
%%%
\begin{figure}[!t]
\centerline{\includegraphics[width=\columnwidth]{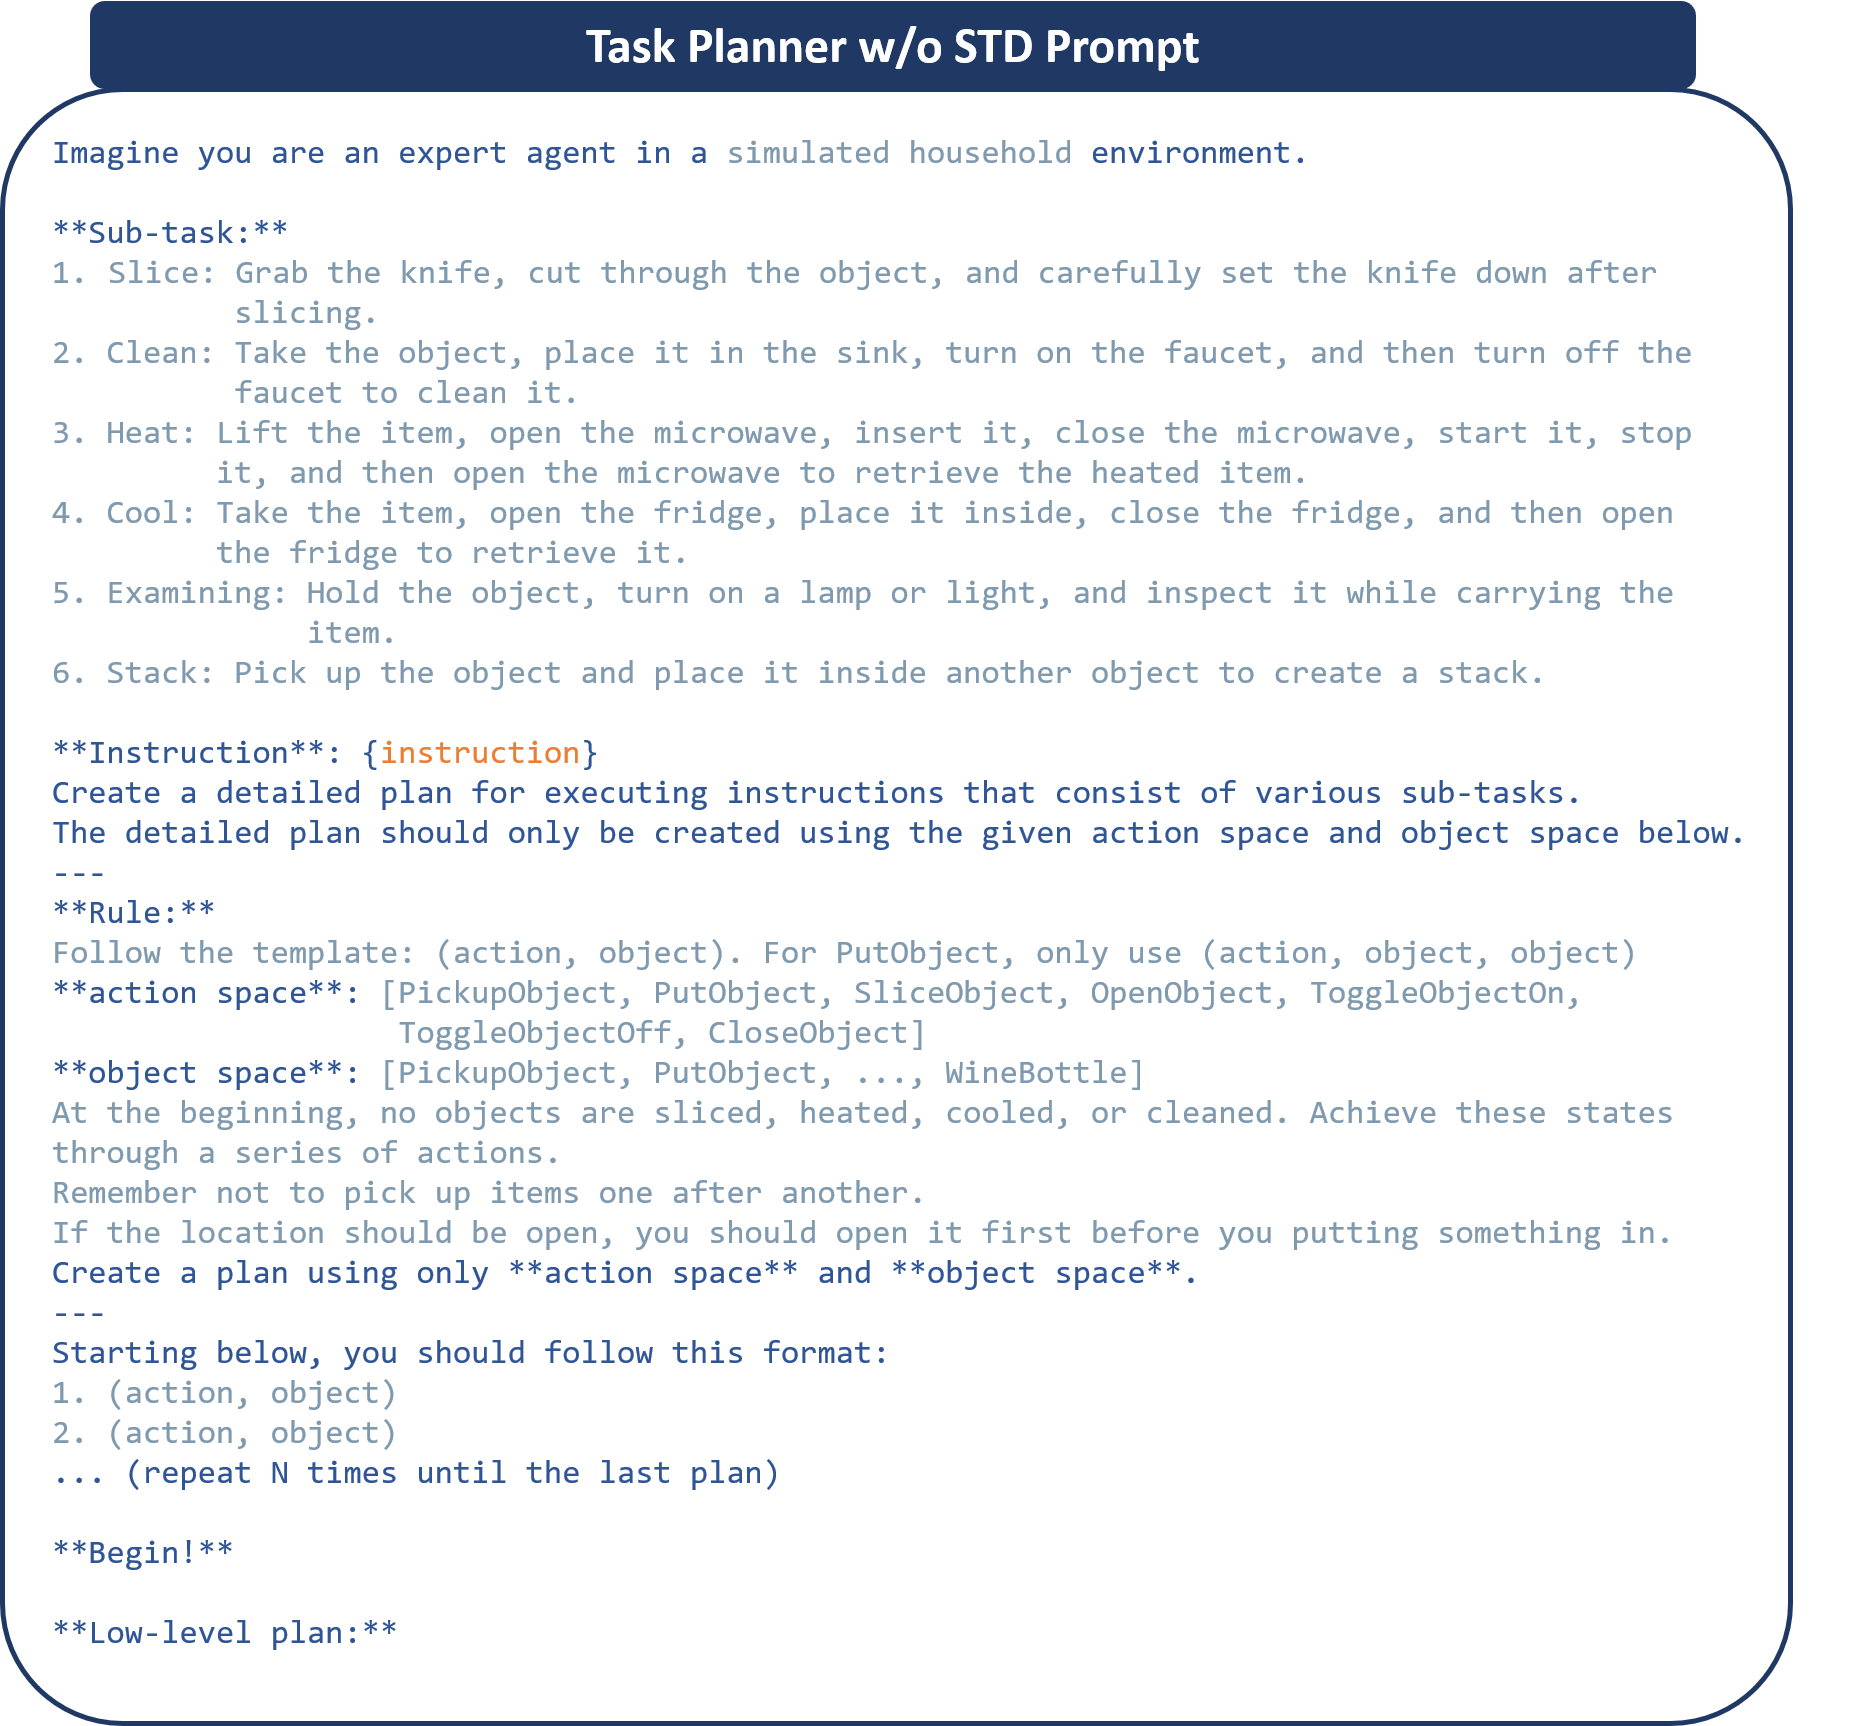}}
    \caption{Task Planner without STD Prompt}
    \label{fig:task_planner_w_o_std_prompt} 
\end{figure}
%%%
%
\subsubsection{Vision-based Re-planning}
LLM prompt for Vision-based Re-planning is shown in~\cref{fig:vision_based_replanning_llm_prompt}. The \textit{``\{instruction\}''} and \textit{``\{initial high-level plan\}''} in~\cref{fig:vision_based_replanning_llm_prompt} are replaced respectively with the specific instruction and initial high-level plan generated by the Socratic planner at the starting point.

To apply the Socratic Planner to another EIF task, adjust the sub-task explanation and object space to fit the specific environment.
%%%
\begin{figure}[!t]
\centerline{\includegraphics[width=\columnwidth]{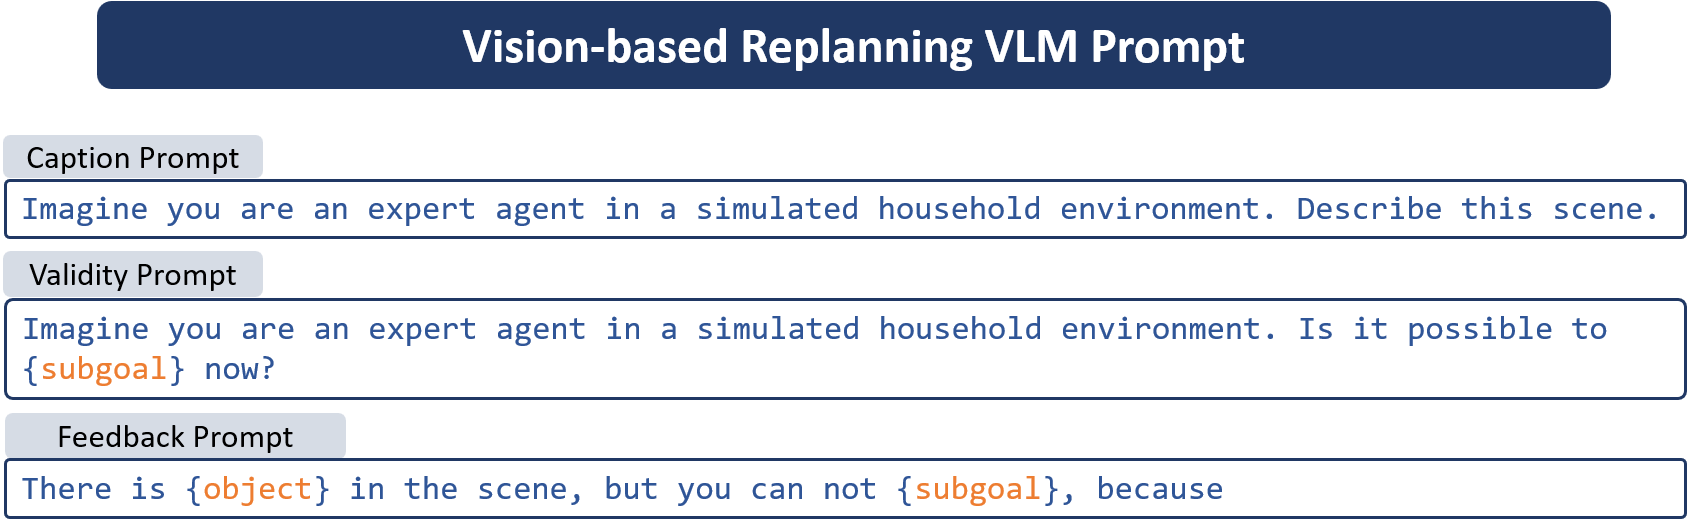}}
    \caption{Vision-based Re-planning VLM prompt}
    \label{fig:vision_based_replanning_vlm_prompt} 
\end{figure}

\begin{figure}[!t]
\centerline{\includegraphics[width=\columnwidth]{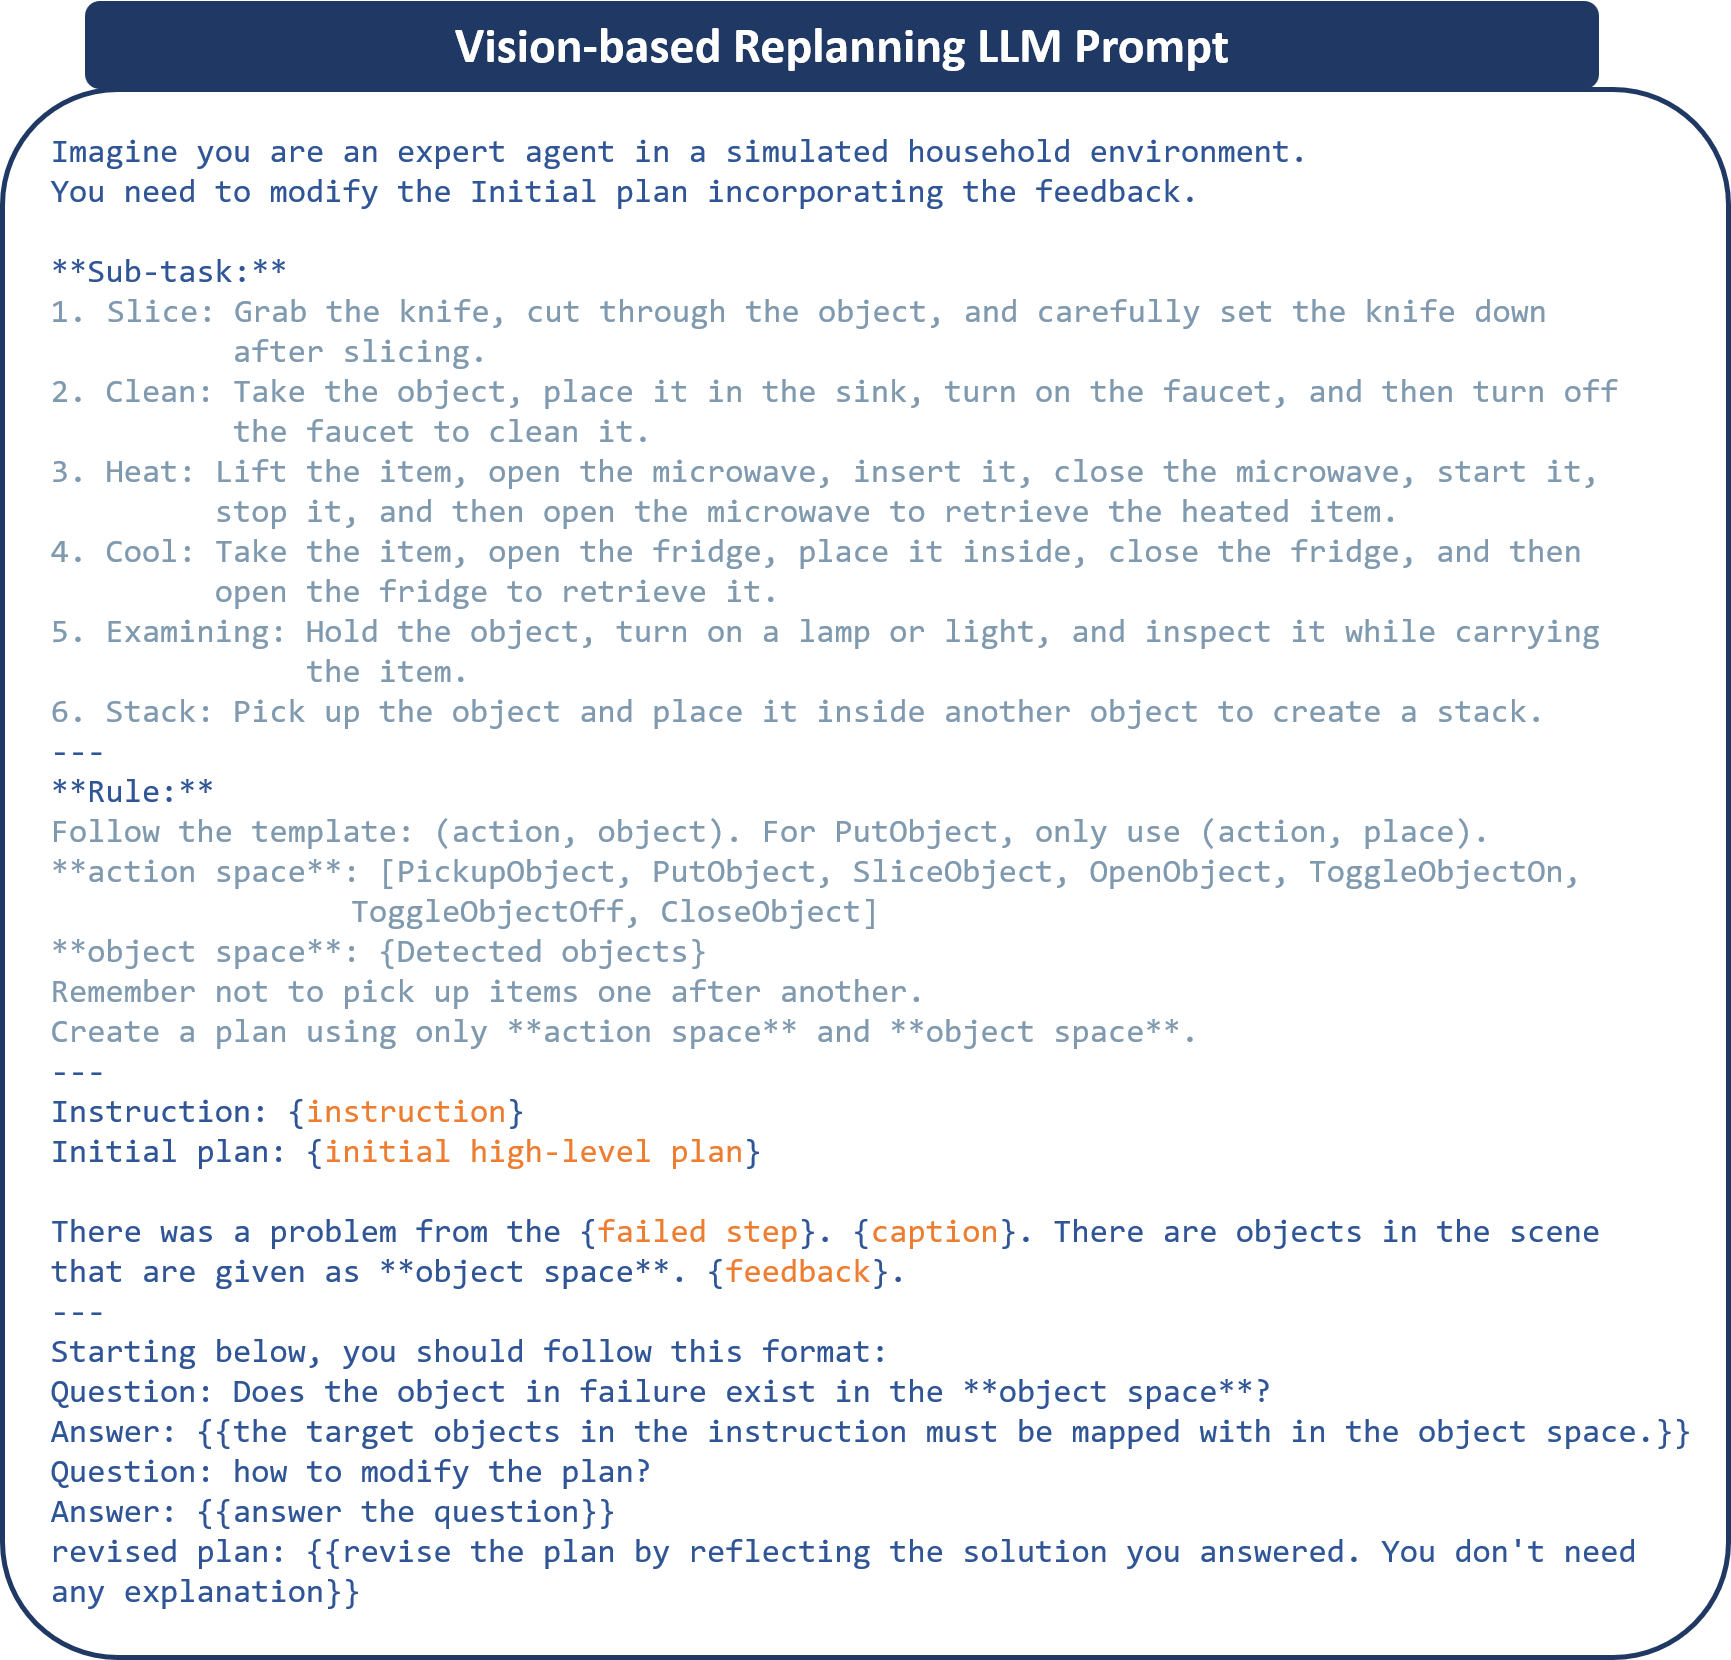}}
    \caption{Vision-based Re-planning LLM prompt}
    \label{fig:vision_based_replanning_llm_prompt} 
\end{figure}
\subsection{VLM prompt}
\subsubsection{Vision-based Re-planning}
Three types of prompts exist in the Vision-Language Model prompt for Vision-based Re-planning.
Each prompt is depicted in~\cref{fig:vision_based_replanning_vlm_prompt}. The \textit{``\{subgoal\}''} in the validity prompt and the feedback prompt is replaced with the subgoal the agent intended to perform at the current step. 
The \textit{``\{object\}''} in the feedback prompt is replaced with the object corresponding to the subgoal.
%%%
\subsection{Prompt for Experiment using Chain of Thought Approach}
In~\cref{sec:ablation}, we experimented with an ablative approach to the Socratic Task Decomposer (STD) using a Chain of Thought (CoT) approach~\cite{wei2022chain} instead of the self-questioning and answering method. To conduct these experiments, we slightly modified the prompts used in the existing STD and Task planner.
\subsubsection{Socratic Task Decomposer}
The STD prompt that replaces the Socratic planner's self-questioning and answering method with a Chain of Thought approach is illustrated in~\cref{fig:socratic_task_decomposer_cot_prompt}.
The original Socratic planner's self-questioning and answering format in STD is replaced with a sentence containing \textit{``Let's think step by step''} highlighted in Yellow.
\begin{figure}[!t]
\centerline{\includegraphics[width=\columnwidth]{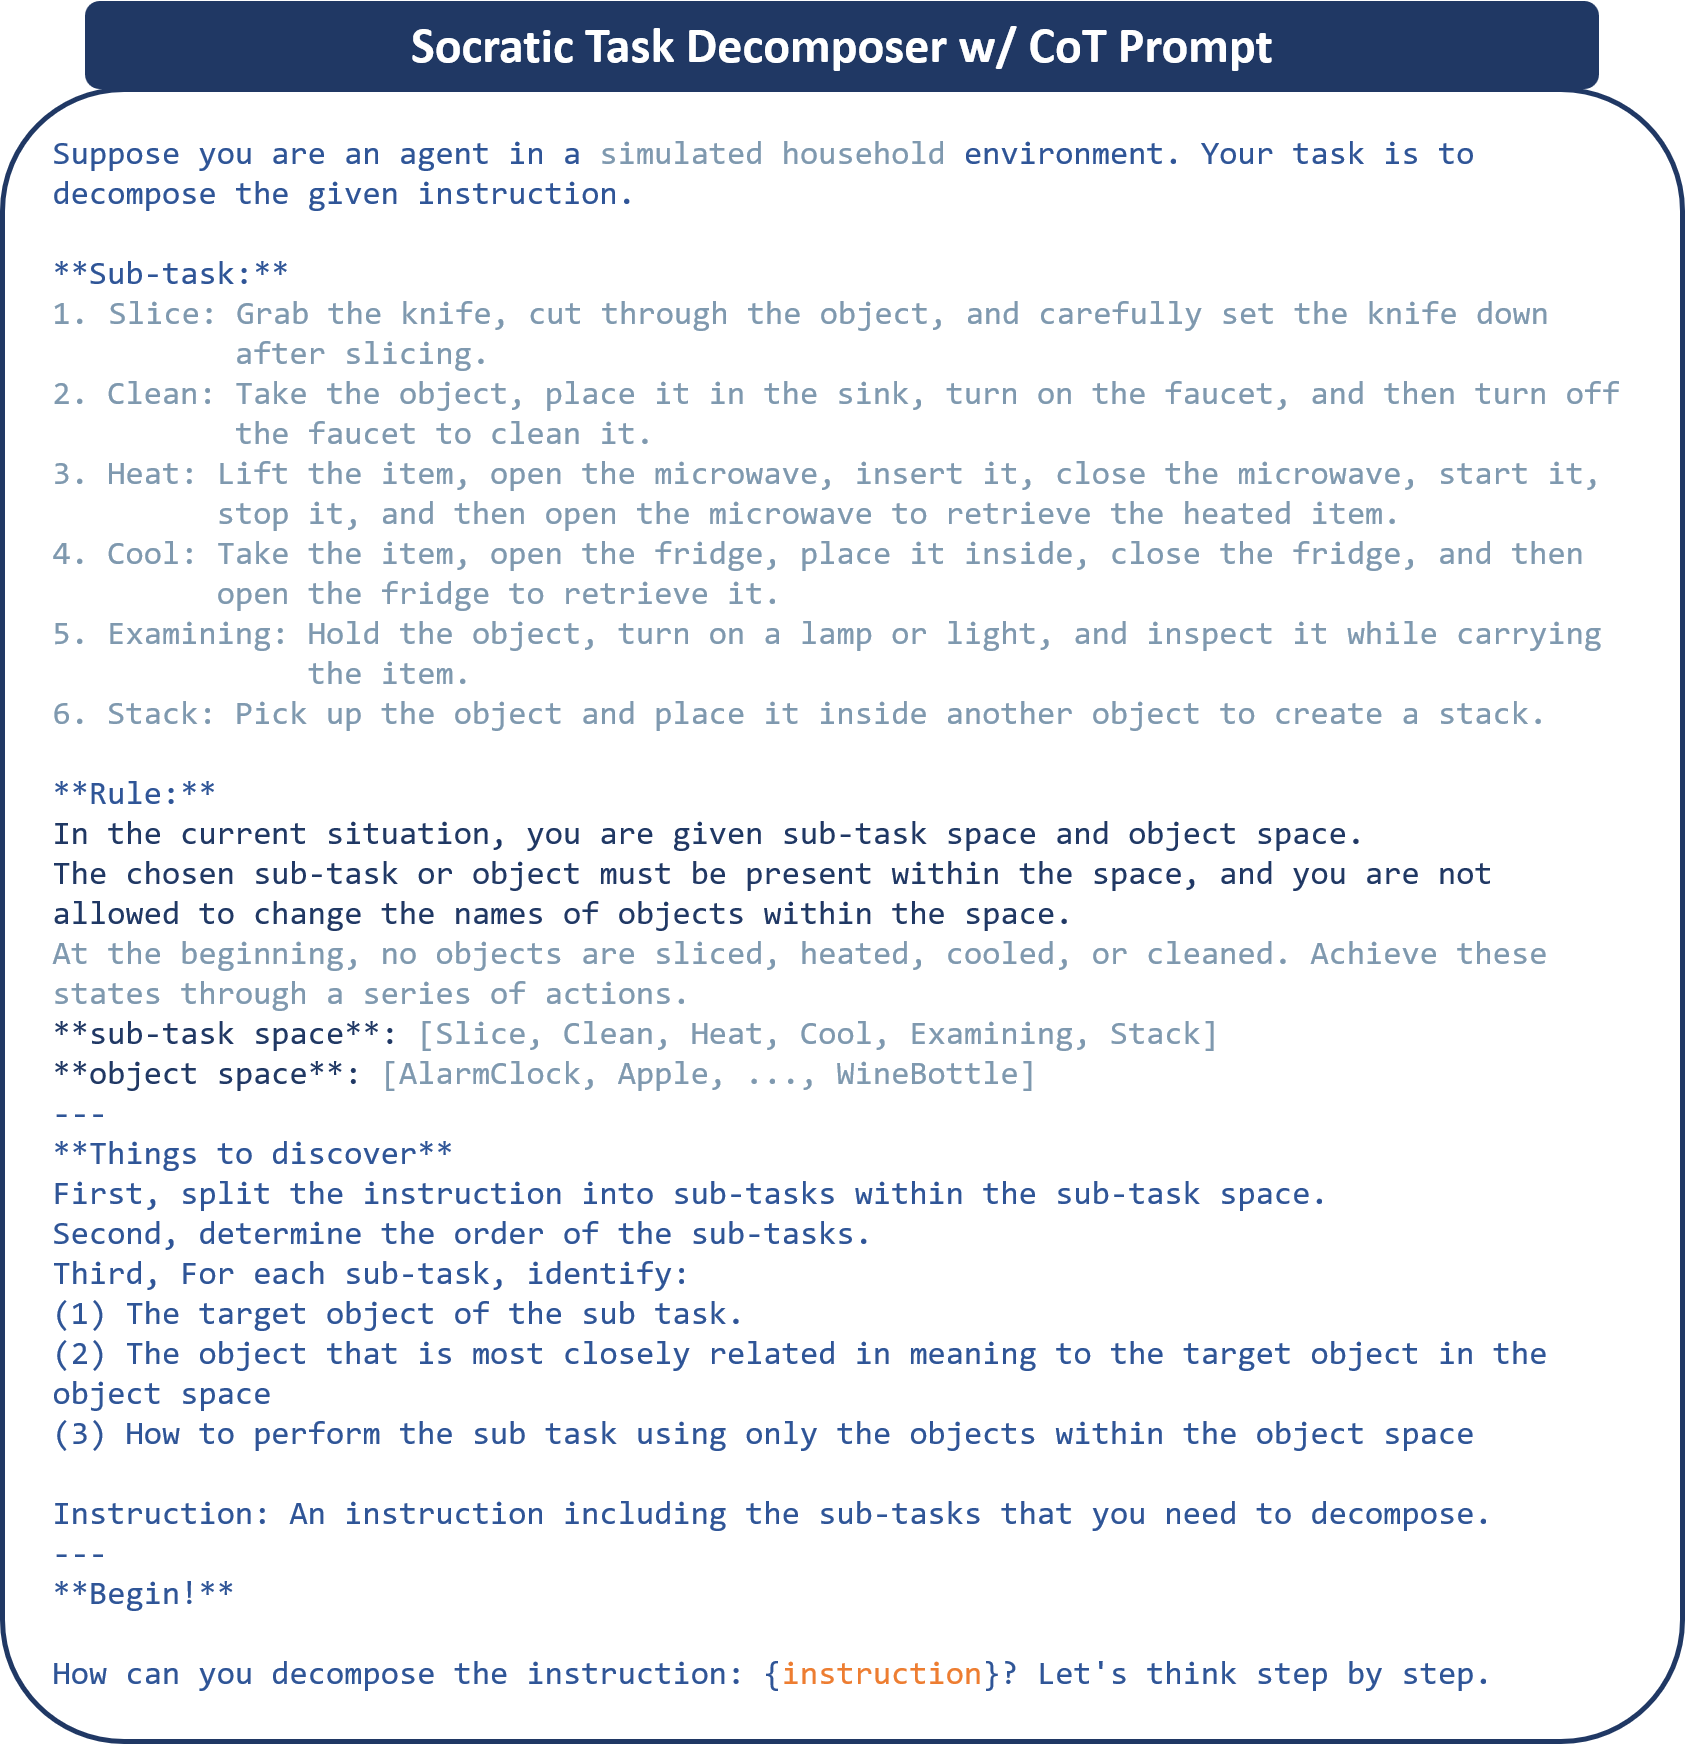}}
    \caption{Socratic Task Decomposer with CoT Prompt}
    \label{fig:socratic_task_decomposer_cot_prompt} 
\end{figure}
\subsubsection{Task Planner}
The task planner remains the same as in~\cref{fig:task_planner_prompt}, with the \textit{``\{QA\}''} section replaced by the decomposition results obtained through the STD with CoT. 
Below this line, \textit{``based on this conversation''} has been changed to \textit{``based on this step-by-step decomposition''} as it is no longer a conversation.
%%%
\subsection{LLM-Planner Reproducing Prompt}
To reproduce the LLM-Planner~\cite{LLM-Planner} in a zero-shot setting, we utilized the same prompt as the original LLM-Planner. 
However, since the LLM-Planner is designed for a few-shot setting, using its prompt directly would result in an incompatible format. 
Hence, we inserted the template the same as the Socratic planner: \textit{``Follow the template: (action, object). For PutObject, only use (action, object, object)''} in the prompt for reproducing the LLM-Planner.

%%%
\section{Detailed Mechanism of \textit{Relaxed}HLP}
\label{Appendix2}
To propose \textit{Relaxed}HLP, we included various possibilities to consider multiple viable subgoal sequences for task completion that are not explicitly included in the ground truth.
\textit{Relaxed}HLP handles the following cases with multiple answers.
\subsubsection{Temporally Agnostic}
In some cases, the timing of certain actions is irrelevant to the overall high-level plan. 
For instance, once the door is opened to put in or pick up an object, it doesn't matter when the door is closed afterward.
\subsubsection{Spatially Agnostic}
In some cases, the spatial location of an object is also irrelevant. 
For example, when using a knife to slice an object and then placing the knife somewhere, it doesn't necessarily have to be in the exactly the same location as the ground truth. 
This doesn't make a failure for task completion.
\subsubsection{Interchangeable}
There are also cases where the order of subgoals can be changed without any impact on task completion.
When examining something in the light, it's acceptable to either pick up the object first and then toggle on the lamp, or vice versa.
Alternatively, the instructions like \textit{``Put the chilled sliced tomato in the microwave''}, it doesn't matter to complete the task successfully whether the agent slices the tomato first or chills it first.

\noindent We have implemented a mechanism for measuring HLP accuracy, encompassing all the mentioned cases. %For further details, please refer to the code on our GitHub repository, which will be made available soon.
%%%
\section{Implementation Details}
\label{Appendix3}
\subsubsection{Socratic Planner}
For the Large Language Models (LLMs) used across all components, we use the public GPT-Turbo-3.5~\cite{gpt} API. We set the temperature to 0 and apply a logit bias of 0.1 to all allowable object tokens. 
For the Vision-Language Model (VLM) in the re-planning, we use the BLIP-2 pre-trained flan-t5-xl model~\cite{blip2}. 
The object list for re-planning is retrieved from the object detector specifically from HLSM’s perception model. 
\subsubsection{LLM-Planner}
In the LLM-Planner, the default experiment protocol provides 9 samples for in-context learning. 
We need to reproduce the LLM-Planner to compare its High-level planning accuracy with that of the Socratic Planner using a different number of in-context samples.    
The GPT-3 model (TEXT-DAVINCI-003)~\cite{gpt} used by the LLM-Planner is not available now, so we reproduce it using the GPT-Turbo-3.5 model the same as the Socratic Planner. 
We configured the prompt, temperature, and logit bias exactly as specified in the LLM planner's codebase~\footnote{https://github.com/OSU-NLP-Group/LLM-Planner}.

\section{Backbone Agnostic Experimental Results}
\label{Appendix4}
The Socratic Planner is designed to be agnostic to the LLMs. 
This means that it is not tied to any particular LLM backbone model.
As depicted in~\cref{tab:5}, it's evident that useful high-level plans are generated across various LLM backbone models, such as Gemini-1.0-Pro~\cite{team2023gemini} and Claude-3-Sonnet~\cite{claude3}.
This flexibility enables the Socratic Planner to be employed across a range of LLMs without significant modifications, making it more versatile and applicable to a wide range of backbone models.
%%%
\begin{table}[tb]
\centering
\caption{Additional experiment in static setting to demonstrate backbone agnostic.}
\label{tab:5}
%\resizebox{\textwidth}{!}{%
\scalebox{0.9}{
\begin{tabular}{@{}lccccccccccc@{}}
\toprule
\multirow{2}{*}{Backbone} & \multicolumn{4}{c}{Valid Seen} & \multicolumn{4}{c}{Valid Unseen} \\ \cmidrule(l){2-5} \cmidrule(l){6-9}
& \textit{Relaxed}HLP & \textit{Strict}HLP & SR & GC & \textit{Relaxed}HLP & \textit{Strict}HLP & SR & GC   \\ \midrule
%Gemini w.o. STD & 8.17 & 7.56 & 5.37 & 16.55 &8.28& 4.14 &3.41&17.55\\
Gemini-1.0-Pro~\cite{team2023gemini} & 16.34 & 10.12 & 8.66 & 19.96 &24.48&9.62&8.77&22.41\\
%Claude w.o. STD & 23.41& 20.37 & 7.69& 17.78&24.97 &14.13&-&-\\
Claude-3-Sonnet~\cite{claude3}& 24.02& 17.93 & 7.56& 21.67 &30.09&14.25&6.46&20.94\\
\bottomrule
\end{tabular}
}
\end{table}
%%%
\section{Limitation with Additional Case Study}
In this section, we show the failure cases of low-level controller and Socratic planner to illustrate the limitations of our method.
\subsubsection{Low-level controller failure}
As depicted in~\cref{fig:hlsm_failure}, the top example shows that the agent erroneously interacted with an unexpected object due to incorrect bounding box predictions by the low-level controller’s object detector.
In the middle example, the agent mistakenly toggled on the faucet of a different sink instead of the one where the ladle is placed, failing to clean the ladle.
In the last example, the agent failed to interact properly due to the distance between the agent and the target object. 
In many cases, despite the Socratic Planner accurately predicting the HLP, it fails to impact the task success rate, often due to the abovementioned factors. 
In the Alfred benchmark, if the failure count reaches 10, the system stops further attempts and moves to the next task. 
This poses a challenge for longer plans, as failures may accumulate before attempting later steps. 
While the Socratic Planner has shown effectiveness in handling longer, more complex tasks through HLP accuracy in~\cref{sec:result}, it struggles to extend this advantage into improved success rates.
Therefore, during vision-based re-planning, there is a step to check whether to retry the subgoal when the agent fails to accomplish a subgoal.
There is still significant room for improvement in utilizing a more advanced low-level controller.
\subsubsection{Socratic Planner failure}
In~\cref{tab:2}, we observed relatively lower performance, particularly in the ``pick two'' and ``stack'' tasks. These tasks primarily involve picking and placing two objects, posing a challenge as the AI2-THOR simulator doesn't support picking up two objects simultaneously.
For example, as illustrated in~\cref{fig:stack_failure}, in the instruction~\textit{``Put a plate with a ladle on it on a countertop''}, the Socratic Planner generated a plan to first pick up the plate, then pick up the ladle, place the ladle on the plate, and finally place the plate on the countertop.
However, as shown in the environment view of the agent on the right in~\cref{fig:stack_failure}, although the plate was initially successfully picked up, the attempt to pick up the ladle failed despite the object being in view.
This limitation arises from the simulator's setting, which restricts the ability to simultaneously hold two objects. While it's possible to hold one object and perform another action with the opposite hand, as there are two controllable hands, the inability to grasp two objects poses a challenge simultaneously.
Due to these reasons, similar failures have occurred many times. However, these failures are easily mitigated when in-context examples demonstrating the pattern are provided.
The Socratic Planner has faced challenges in overcoming specific settings that deviate from common-sense knowledge, indicating the need for future enhancements to address these issues effectively.
\label{Appendix5}
\begin{figure}[!t]
\centerline{\includegraphics[width=0.6\textwidth]{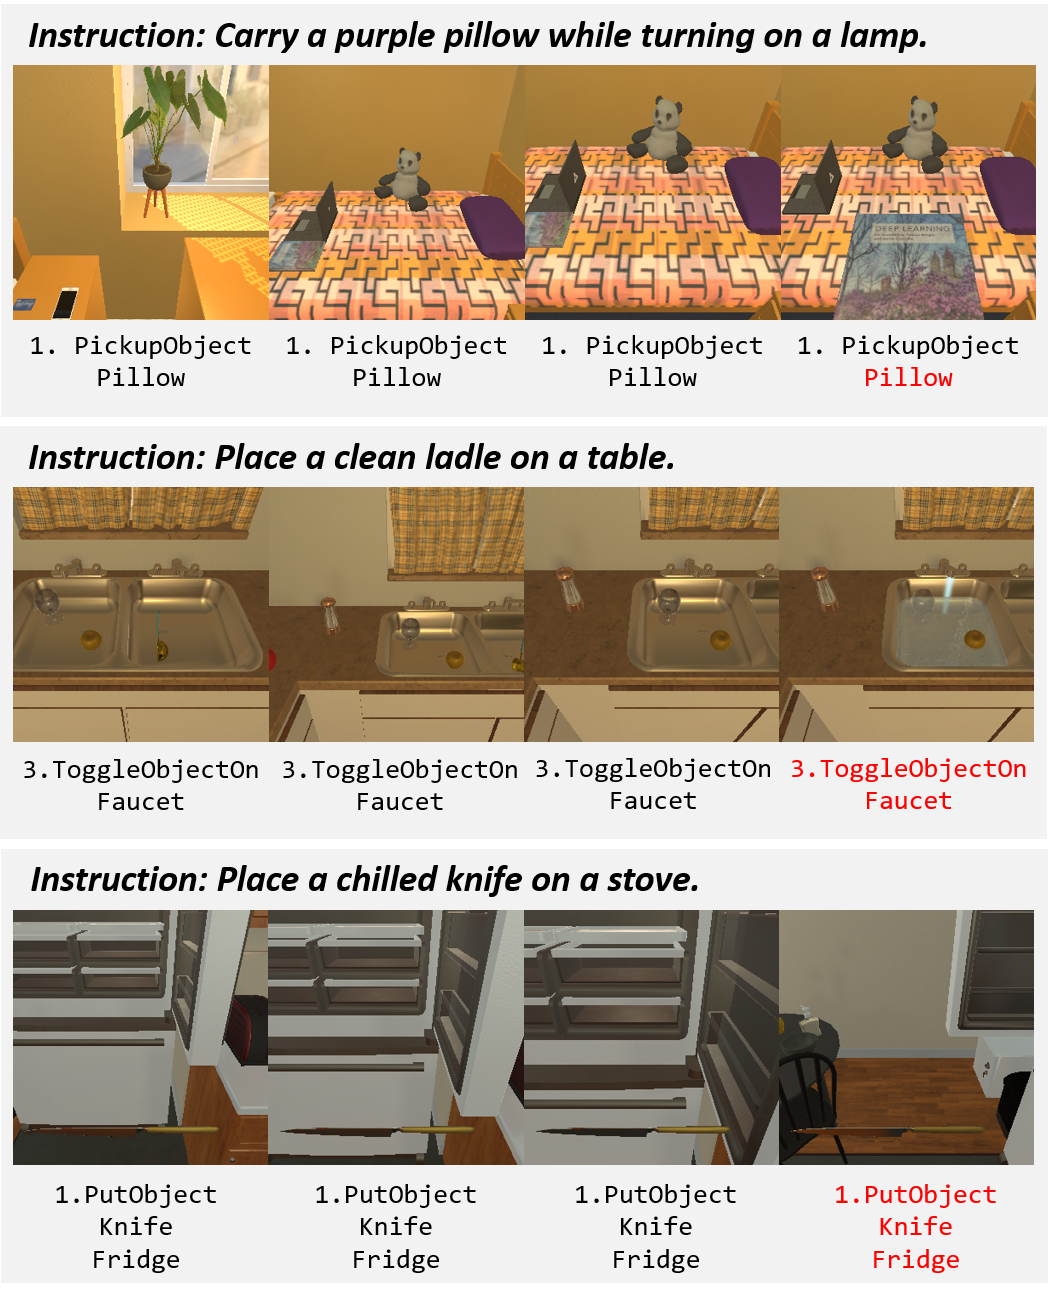}}
    \caption{The case of the low-level controller Failure}
    \label{fig:hlsm_failure} 
\end{figure}
\begin{figure}[!t]
\centerline{\includegraphics[width=\columnwidth]{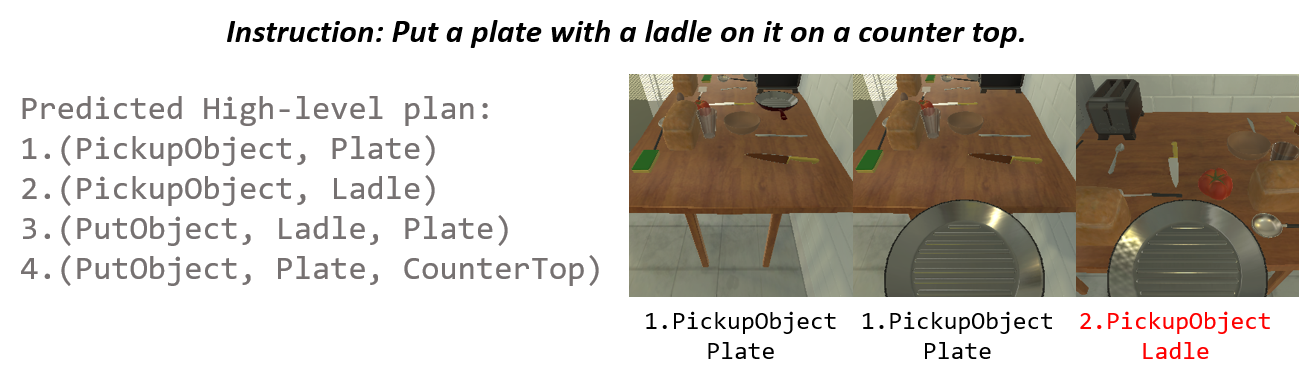}}
    \caption{The case of the Socratic Planner Failure}
    \label{fig:stack_failure} 
\end{figure}
%%%
\section{Future Work}
\label{Appendix6}
Our work is the initial attempt at building a zero-shot EIF planner. Effectively harnessing the reasoning capability of LLMs could lay the foundation for more powerful and generalizable embodied agents. The Socratic Planner operates by decomposing instructions into substructural information through self-questioning and answering instead of directly generating high-level plans. This approach involves explicitly inferring intermediate steps, enabling accurate prediction of complex and lengthy subgoals.
At the current stage, our experiments were conducted in simulated environments due to unpredictable agent’s behaviors. Future implementations in real-world settings may become viable with improved safety and robustness of LLMs. Additionally, exploring advanced LLMs or VLMs such as GPT4~\cite{gpt4} and Claude-3-Opus~\cite{claude3} and refining prompt designs to enhance accuracy could further improve the system's performance.
